# Supplementary material for: Self-Organized Critical Coexistence Phase in Repulsive Active Particles
Source: arXiv:2007.03587 ancillary file (2021-01-26)
Supplement: Supplementary file 1 [file SupplementaryInformation.pdf]

# Supplementary Information for: "Self-Organized Critical Coexistence Phase in Repulsive Active Particles"

Xia-qing Shi,[1,2] Giordano Fausti,[2] Hugues Chaté,[2,3,4] Cesare Nardini,[2] and Alexandre Solon[4]

[1] *Center for Soft Condensed Matter Physics and Interdisciplinary Research, Soochow University, Suzhou 215006, China*
[2] *Service de Physique de l'Etat Condensé, CEA, CNRS Université Paris-Saclay, CEA-Saclay, 91191 Gif-sur-Yvette, France*
[3] *Computational Science Research Center, Beijing 100094, China*
[4] *Sorbonne Université, CNRS, Laboratoire de Physique Théorique de la Matière Condensée, LPTMC, F-75005 Paris, France*

## Numerical details about ABPs

Active Brownian particles are simulated using a simple Euler scheme, with timestep $dt = 0.02$. We roughly scanned parameter space, noticing that bubbles are more prominent/persistent with anisotropic motility/noise. Initially, particles are randomly distributed in a band occupying a $\rho_0$ fraction of the system. This shortens the transient leading to (band) steady-state. Transients are then estimated by looking at timeseries of total bubble area.

*Detection of bubbles:* We first build a coarse-grained density field by calculating local packing fraction in $2\sigma \times 2\sigma$ boxes. (Fig. 1(a,b) of the main text shows a typical result.) We then detect its contour lines at a chosen threshold $\rho^*$. We can then calculate bubble areas. All data shown in the main text were collected using $\rho^* = 0.7$. We checked that other reasonable choices of $\rho^*$ do not change our results significantly.

## Numerical details about our active lattice gas

Particles live on an hexagonal lattice, and perform synchronously one of three basic moves, as illustrated in Fig. 1(a): 'self-propelled' jump along their polarity direction at rate $r_P$, spatial diffusion to any neighboring site at rate $r_D$, or rotational diffusion (changing their polarity to one of its two neighboring orientations) at rate $r_R$. We impose strict exclusion in the model, and use parallel updating. at each timestep, all particles are simultaneously updated according to trial probabilities $p_P = r_P/p_0$, $p_D = r_D/p_0$ and $p_R = r_R/p_0$, where $p_0 = r_P + r_D + r_R$. The chosen move is canceled if the target site is already occupied. If several particles want to move to the same empty site, we draw an additional random number to select which of them will move and the others remain on location. We checked that the usual random updating gives very similar results (at the same basic rates). On a single processor, the parallel update model is about 5 times faster than the random update version. Moreover, parallel updating means that the model can be easily simulated on a parallel computer.

Bubbles are ubiquitous in this model, but a brief scan of parameter space was first conducted to locate a phase coexistence regime with prominent ones. Initial conditions: To study bubbles in band phase coexistence, we put all the particles randomly in a given band slab occupying about a $1.1\rho_0$ fraction of the simulation domain. Transients (typically of $10^8$ timesteps) were discarded after inspection of the times series of bubble fraction $\phi_b$. To study coarsening and to study the microphase-separated steady-states at high $\rho_0$, we just distribute particles at random. Bubble detection was performed like in the case of ABPs: a coarse-grained density field (taking discrete

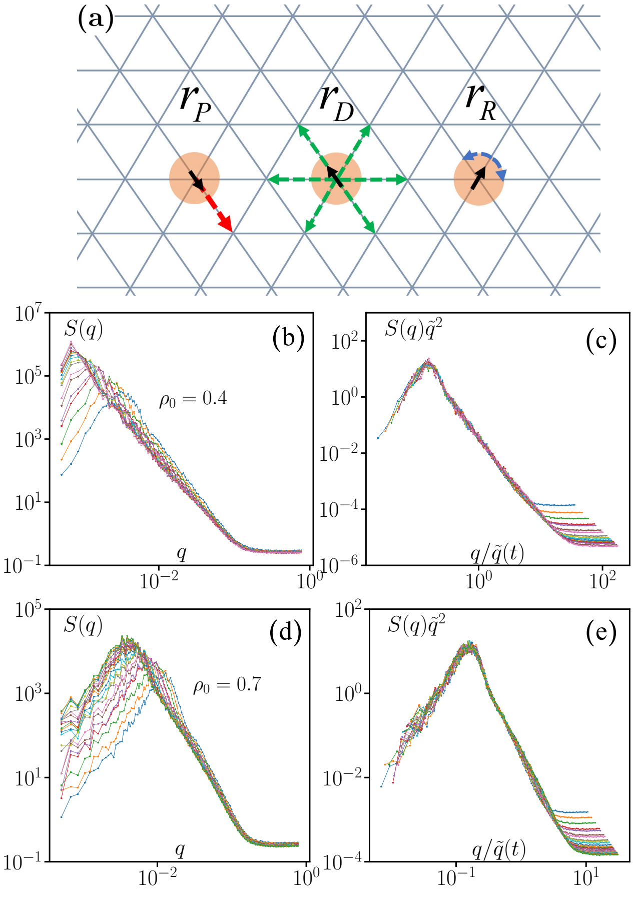


FIG. 1. Active lattice gas model. (a) Schematic diagram describing the three moves attempted by particles. The black arrows indicate the polarity of the particle. Streaming along polarity (red arrow) occurs at rate $r_P$, spatial diffusion at rate $r_D$ (green arrows), and rotational diffusion at rate $r_R$ (blue arrows). (b-e): Structure factors calculated along the runs presented in Fig. 6 of the main text. (b,d): instantaneous structure factor at various times from $t = 10^5$ to $t = 10^7$. (c,e): same as (b,d), but rescaled by $\tilde{q}$. ($\rho_0 = 0.4$ in (b,c), $\rho_0 = 0.7$ in (d,e)).

values here) was calculated in $2 \times 2$ boxes. Contour lines at a given threshold $\rho^*$ were constructed.

### Measurements during coarsening

To measure the characteristic length scale $\tilde{L}(t)$ in the active lattice gas as shown in Fig. 6 of the main text, we also use the density field coarse-grained on $2 \times 2$ boxes, which have a $2 : \sqrt{3}$ aspect ratio since we are dealing with an hexagonal lattice. We then Fourier transform this density field and obtain a 2D discretized static structure factor $S(q_i, q_j)$. Performing an angular averaging, we obtain the discretized $S(q)$ shown in Fig. 1(a,c) at various times. The first moment of the static structure factor $\tilde{q}$ can then be obtained by averaging over this discretized structure factor. To check if the power-law growth regime follows the dynamic scaling hypothesis, we rescale $q$ with the characteristic wave number $\tilde{q}$ and $S(q)$ with $\tilde{q}^{-2}$. For each of the powerlaw growth regimes shown at different densities $\rho_0$ in Fig. 6 of the main text, the rescaled structure factors collapse very well, as shown for two cases in Fig. 1(b,d).

### Numerical details about the reduced bubble model

Each bubble, assumed to be perfectly circular, is characterized by its position and radius $r$. We performed simulations in two geometries: periodic boundary conditions (as in Fig.4c, main text) and within a band of liquid (as in Fig.4a, main text). Let us first describe the algorithm for periodic boundary conditions.

During a timestep $dt = 0.1$, the following actions are performed:

- New bubbles of radius $r_0 = 1$ are nucleated in the liquid. The number of new bubbles is given by $N_{\text{new}} = \lfloor k_n x_\ell S dt \rfloor + \xi$ where $S = L_x \times L_y$ is the system size, $x_\ell$ the fraction of liquid. $\xi$ is a random number which takes value 1 with probability $k_n x_\ell S dt - \lfloor k_n x_\ell S dt \rfloor$ and 0 otherwise.
- The area of all bubbles shrink by an amount $\kappa r(1 - r/r_0)$ with $\kappa$ computed so that the area of gas is exactly conserved.
- We perform a random sequential update of the position of the bubbles: We choose bubble $i$ at random, add diffusion to its position $(x_i, y_i)$, $x_i(t + dt) = x_i(t) + \sqrt{2Ddt}\eta_x$ (and similarly for the $y$ component) with $\eta_x$ a random Gaussian number with unit variance. If the bubble overlaps with another one, they coalesce while conserving the total area. The resulting bubble is placed at the center of mass of the two merging ones. During the timestep, we update $n(t)$ bubbles where $n(t)$ is the number of bubbles after the nucleation step.

In the band geometry, we follow in addition the edges of the outside gas phase. It shrinks with a rate $\kappa L_y$ on each side (*i.e.* proportional to the length of the interface, like bubbles). If a bubble touches one of the boundaries, the bubble disappears and the boundary moves such that the gas area is conserved. No diffusion is applied on the edges. The simulation ends if the size of the outside gas vanishes.
